# Supplementary material for: Efficient-Adam: Communication-Efficient Distributed Adam
Source: arXiv:2205.14473 source file (2023-08-24)
Supplement: Supplementary file 1 [file supplementary_compressor.tex]

\section{Generalized to Compressor}

In this section, we will analyze the converge property of above algorithms. To analyze the converge of the above algorithms we need some more assumptions on quantization functions and hyper-parameter choice.

\begin{assumption}
\label{A2}
For the quantization function used in Algorithm \ref{alg1}, there exists a positive value $\delta_x$, such that the inequality holds: $\|x-Q_x(x)\|\leq (1-\delta_x)\|x\|$.
\end{assumption}

Similarly, we have the addition assumption for the quantization function in Algorithm \ref{alg2}.

\begin{assumption}
\label{A3}
For the quantization function used in Algorithm \ref{alg2}, there exists a positive value $\delta_g$, such that the inequality holds:
$\|x-Q_g(x)\| \leq (1-\delta_g)\|x\|$.
\end{assumption}

In addition, we make the following assumption on momentum average parameter $\beta$, exponential moving average parameter $\theta_t$ and learning rate $\alpha_t$.

\begin{assumption}\label{A4}
We assume that $\theta_t = 1-\frac{\theta}{t}$, and $\alpha_t = \frac{\alpha}{\sqrt{t}}$. Besides, we choose $\theta'$ such that $0<\beta^2<\theta'<1$ and denote $\gamma = \beta/\theta'$. Let $n = max\{j|\theta_j<\theta'\}$, then we denote $C_1 = \prod_{j=1}^n \frac{\theta_j}{\theta'}$.
\end{assumption}

\subsubsection{Single Worker Analysis}
  In this section, we establish the convergence result for single worker. Because there is only one worker, there is not average operation in the algorithm. We can view the composition of 2 quantization functions as one quantization function. For simplicity, we use $Q_g(x)$ to represent the compound function and use $\delta_g$ as the quantization error defined similarly in the Assumption \ref{a3}. 
  
\begin{theorem}
\label{T1}
Let $\{x_t\}$ be the sequence generated by Algorithm \ref{alg1} and Algorithm \ref{alg2}.
In addition, let $x_\tau^T$ represent random variable $x_\tau$ with $\tau$ taking from $\{1,2,\ldots,T\}$ with the same probability. The convergence result holds as follows: 
\begin{equation}
(E[\|\nabla f((x_\tau^T))\|^2]) \leq \frac{C+C'\sum_{t=1}^T\frac{1}{t}}{\sqrt{T}},
\end{equation}
where  $ C_2 = \left(\frac{\beta/(1-\beta)}{\sqrt{C_1(1-\gamma)\theta_1}}+1\right)^2$, $C_3 = \frac{1}{\sqrt{C_1}(1-\sqrt{\gamma})} \left(\frac{\alpha L(2-\delta_g)}{C_1\theta(1-\sqrt{\gamma})^2\delta_g} + \frac{2C_2G}{\sqrt{\theta}} \right)$, 
    $C = \frac{2\sqrt{G^2+\epsilon d}}{(1-\beta)}\left(f(x_1)-f^*+ \alpha C_3d\log\left(1+\frac{G^2}{\epsilon d}\right)\right)$, and, 
    $C' = \frac{2\sqrt{G^2+\epsilon d}C_3d}{(1-\beta)(1-\theta)}$.
\end{theorem}
The proof of Theorem \ref{T1} can be seen in Section \ref{pft1}. 
From this result, it can be seen that with quantization error will hurt the convergence speed by effect constant $C_3$. This result can reduce to the origin Adam's convergence rate when $\delta_g$ goes to 1, which means no error in quantization. Besides, the order of convergence rate does not hurt by adding quantization, it is still $O(\log(T)/\sqrt{T})$.

\subsubsection{Multi-Worker Analysis}
In this section, we consider multi-worker setting. We denote the number of workers as $N$, and make additional assumption that all workers works identically and independently, i.e. $\xi$ on each worker follows the same distribution and is independent to each other.

\begin{theorem}
\label{T2}
 Let $\{x_{t}\}$ be the point generated by Algorithms \ref{alg1} and Algorithm \ref{alg2}. 
 In addition, let $x^T_\tau$ be the random variable $x_\tau$ with $\tau$ taking from $\{1,2,\ldots,T\}$ with the same probability. the convergence result holds as follows:  
 \[
\mathbb{E}[\|\nabla f(x_\tau)\|^2]\leq \frac{C_5+C_6\sum_{t=1}^T \frac{1}{t}}{\sqrt{T}},
\]
where $C_2 = \left(\frac{\beta/(1-\beta)}{\sqrt{C_1(1-\gamma)\theta_1}}+1\right)^2$,
$C_4 = \frac{1}{\sqrt{C_1}(1-\sqrt{\gamma})} \left(\frac{\alpha L(2-\delta_x)(2-\delta_g)}{C_1\theta(1-\sqrt{\gamma})^2\delta_x\delta_g} + \frac{2C_2G}{\sqrt{\theta}}\right)$,
$C_5 = \frac{2\sqrt{G^2+\epsilon d}}{\alpha(1-\beta)}\left(f(x_1) - f^* + C_4d\alpha\log\left(1+\frac{G}{\epsilon d}\right)\right),$ and, $C_6 = \frac{2\sqrt{G^2+\epsilon d}C_4 d}{(1-\beta)(1-\theta)}$.

\end{theorem}

The proof of Theorem \ref{T2} is in Section \ref{pft2}. From this result it can be shown that when $delta_x$ goes to 1 or $\delta_g$ goes to 1 the theorem will reduce to Theorem \ref{T1}. And still the convergence rate will not be hurt by adding both direction quantization and quantization error will affect the constant $C_4$ which will effect the speed of convergence in the constant level.

\subsection{Proof of Theorem 1}\label{pft1}
To prove Theorem \ref{T1}, more useful notations and lemmas are needed. So we first introduce some notations in this section. Because there is only one worker, for simplicity, we denote $m_t$, $v_t$ as $m_t^{(1)}$, $v_t^{(1)}$, respectively.notations
\begin{notation}\label{notation-thm1}
Let $\mathbb{E}_t(\cdot) = \mathbb{E}_\xi(\cdot|x_t)$. 
Denote 
$\sigma^2_t = \mathbb{E}_t(g_t^2)$, 
$\hat{v}_t = \theta_t v_t + (1-\theta_t) \sigma^2_t$, 
$\hat{\eta}_t = \alpha_t/\sqrt{\hat{\theta}_t}$, 
$\Delta_t = -\alpha_t m_t/\sqrt{v_t}$, 
$M_t = \mathbb{E}[\langle\nabla f(x_t), \Delta_t\rangle+L(2-\delta_g)\|\Delta_t\|^2 + L(2-\delta_g)\|e_t\|\|\Delta_t\|]$,
 and $\|x\|_{\hat{\eta}_t}^2 = \sum_{i=1}^d \hat{\eta}_t^{(i)}{x^{(i)}}^2$.
In addition, let $\tilde{x}_t = x_t - e_{t}$. Then, it holds that  $\tilde{x}_{t+1} = x_t - Q_g(-\Delta_t+e_t) - e_{t+1} = x_t + \Delta_t -e_t = \tilde{x}_t + \Delta_t$.
\end{notation}

\begin{lemma}\label{Lemmamv}
By using Notation \ref{notation-thm1} and the iteration scheme of Theorem 1, for all $t\ge 1$ the following inequality holds:
\[
  m_t^2\leq \frac{1}{C_1(1-\gamma)(1-\theta_t)}v_t.
\]
\end{lemma}
\begin{proof}
By using the definition of $m_t$ in Theorem 1, it directly holds that
\begin{align}\label{eq-mt}
m_t = \sum_{i=1}^t\beta^{t-i}(1-\beta)g_i.
\end{align}
Let $\Theta(t,i) = \prod_{j=i+1}^t \theta_j$ for $i < t$, and $\Theta(i,i) = 1$. According to the definition of $v_t$, it holds that
\[
   v_t = \sum_{i = 1}^t \left(\prod_{j=i+1}^t\theta_j\right)(1-\theta_i)g_i^2 = \sum_{i = 1}^t\Theta(t,i)(1-\theta_i)g_i^2.
\]
With arithmetic inequality and Eq.~\eqref{eq-mt}, it holds that
\[
\begin{split}
    m_t^2 &= \left(\sum_{i=1}^t\frac{\beta^{t-i}(1-\beta)}{\sqrt{\Theta(t,i)(1-\theta_i)}}\sqrt{\Theta(t,i)(1-\theta_i)}g_i \right)^2
    \leq \sum_{i=1}^t\frac{\beta^{2(t-i)}(1-\beta)^2}{\Theta(t,i)(1-\theta_i)}\sum_{i=1}^t\Theta(t,i)(1-\theta_i)g_i^2\\
    &= \sum_{i=1}^t\frac{\beta^{2(t-i)}(1-\beta)^2}{\Theta(t,i)(1-\theta_i)}v_t
    \leq \sum_{i=1}^t\frac{\beta^{2(t-i)}}{(\prod_{j=i+1}^N\theta_j){\theta'}^{t-N}(1-\theta_i)}v_t
    = \sum_{i=1}^t\frac{\beta^{2(t-i)}}{(\prod_{j=i+1}^N\theta_j/\theta')(\theta')^{t-i}(1-\theta_i)}v_t\\
    &\leq \sum_{i=1}^t\frac{\beta^{2(t-i)}}{(\prod_{j=1}^N\theta_j/\theta')(\theta')^{t-i}(1-\theta_i)}v_t
    = \sum_{i=1}^t\frac{\beta^{2(t-i)}}{C_1(\theta')^{t-i}(1-\theta_i)}v_t
    \leq \frac{1}{C_1(1-\theta_t)}\sum_{i=1}^t \left(\frac{\beta^2}{\theta'}\right)^{t-i}v_t\\
    &\leq \frac{1}{C_1(1-\gamma)(1-\theta_t)}v_t.
\end{split}
\]
Then, we obtain the targeted result. 
\end{proof}

\begin{lemma}\label{ft}
  Let $\tau$ be randomly chosen from $\{1,2,\cdots,T\}$ with equal probabilities $p_\tau = \frac{1}{T}$. We have the following estimate:
  \[
  \mathbb{E}[\|\nabla f((x_\tau))\|^2]\leq \frac{\sqrt{G^2+\epsilon d}}{\alpha\sqrt{T}}\mathbb{E}\left[\sum_{t=1}^T\|\nabla f((x_t))\|_{\hat{\eta_t}}^2\right].
  \]
\end{lemma}
\begin{proof}
Note that $\|\hat{v}_t\|_1 = \theta_t \|v_{t-1}\|_1 +(1-\theta_t) \|\sigma_t\|^2$ and $\|g_t\|\leq G$. It is straightforward to prove $\|v_t\|_1 \leq G^2$. Hence, we have $\|\hat{v}_t + \epsilon\|_1 \leq G^2 + \epsilon d$. Utilizing this inequality, we have
\[
\begin{split}
     \|\nabla f(x_t)\|^2 &= \frac{\|\nabla f(x_t)\|^2}{\sqrt{\|\hat{v}_t+\epsilon\|_1}}\sqrt{\|\hat{v}_t+\epsilon\|_1} = \sqrt{\|\hat{v}_t +\epsilon \|_1}\sum_{k=1}^d\frac{|\nabla_k f(x_t)|^2}{\sqrt{\sum_{l=1}^d \hat{v}_{t,l}+\epsilon}}\\
     &\leq \sqrt{\|\hat{v}_t+\epsilon\|_1}\alpha_t^{-1}\sum_{k=1}^d \frac{\alpha_t}{\sqrt{\hat{v}_{t,k}+\epsilon}}|\nabla_k f(x_t)|^2 \\
     &= \sqrt{\|\hat{v}_t+\epsilon\|_1}\alpha_t^{-1}\|\nabla f(x_t)\|_{\hat{\eta}_t}^2 \leq \sqrt{G^2+\epsilon d}\alpha_t^{-1}\|\nabla f(x_t)\|_{\hat{\eta}_t}^2\\
     &\leq \frac{\sqrt{G^2 + \epsilon d}}{\alpha_T}\|\nabla f(x_t)\|^2_{\hat{\eta}_t}.
\end{split}
\]
Then, by using the definition of $x_{\tau}$, we obtain
\[
     \mathbb{E}\left[\|\nabla f(x_\tau)\|^2\right] = \frac{1}{T}\sum_{t=1}^T\mathbb{E}\left[\|\nabla f(x_t)\|^2\right] \leq \frac{\sqrt{G^2 + \epsilon d}}{\alpha\sqrt{T}} \mathbb{E}\left[\sum_{t=1}^T \|\nabla f(x_t)\|^2_{\hat{\eta}_t}\right].
\]
Thus, the desired result is obtained. 
\end{proof}

\begin{lemma}\label{sumdelta}
By using Notation\ref{notation-thm1}, the following inequality holds:
\[
\sum_{i=1}^T \|\Delta_t\|^2 \leq \frac{\alpha^2}{C_1\theta(1-\sqrt{\gamma})^2}\sum_{t=1}^T\left\|\frac{\sqrt{1-\theta_t}g_t}{\sqrt{v_t}}\right\|^2
\]
\end{lemma}
\begin{proof}
By the definition of $m_t$, we can obtain
\[
|m_t| = \left|\sum_{i=1}^t \beta^{t-i}(1-\beta)g_i\right|\leq \sum_{i=1}^t \beta^{t-i}|g_i|.
\]

Because $v_t \geq \theta_t v_{t-1}$, we can easily obtain that $v_t \geq \Theta(t,i) v_i$, where $\Theta(t,i)$ is defined in Lemma \ref{Lemmamv}.

Besides, by using the definition of $\theta'$ in Assumption \ref{A4}, we can obtain
\[
\Theta(t,i) = \prod_{j=i+1}^t \theta_j  \geq (\theta')^{t-n}\prod_{j=i+1}^n \theta_j =(\theta')^{t-i}\prod_{j=i+1}^n (\theta_j/\theta') \geq (\theta')^{t-i}\prod_{j=1}^n (\theta_j/\theta') = C_1 \theta'^{t-i}.
\]

Therefore, we obtain $v_t\geq C_1(\theta')^{t-i}v_i$.

By using the definition of $\Delta_t$, we can obtain
\[
\begin{split}
\|\Delta_t\|^2 &= \left\|\frac{\alpha_t m_t}{\sqrt{v_t}}\right\|^2 \leq \alpha_t^2 \sum_{i=1}^t \left\|\frac{\beta^{t-i}|g_i|}{\sqrt{v_t}}\right\|^2\leq \frac{\alpha_t^2}{(1-\theta_t)C_1} \sum_{i=1}^t\left\|\left(\frac{\beta}{\sqrt{\theta'}}\right)^{t-i} \frac{\sqrt{1-\theta_t} |g_i|}{\sqrt{v_t}}\right\|^2\\
&\leq \frac{\alpha^2}{C_1\theta}\sum_{i=1}^t\left\|\sqrt{\gamma}^{t-i}\frac{\sqrt{1-\theta_i}|g_i|}{\sqrt{v_i}}\right\|^2 \leq \frac{\alpha^2}{C_1\theta}(\sum_{i=1}^t\sqrt{\gamma}^{t-i})\sum_{i=1}^t \sqrt{\gamma}^{t-i}\left\|\frac{\sqrt{1-\theta_i}g_i}{\sqrt{v_i}}\right\|^2\\
&\leq \frac{\alpha^2}{C_1\theta(1-\sqrt{\gamma})}\sum_{i=1}^t \sqrt{\gamma}^{t-i}\left\|\frac{\sqrt{1-\theta_i}g_i}{\sqrt{v_i}}\right\|^2
\end{split}
\]

Hence, it follows that
\[
\begin{split}
\sum_{t=1}^T\|\Delta_t\|^2 &\leq \frac{\alpha^2}{C_1\theta(1-\sqrt{\gamma})}\sum_{t=1}^T\sum_{i=1}^t \sqrt{\gamma}^{t-i}\left\|\frac{\sqrt{1-\theta_i}g_i}{\sqrt{v_i}}\right\|^2 \\
& = \frac{\alpha^2}{C_1\theta(1-\sqrt{\gamma})}\sum_{i=1}^T \sum_{t=i}^T \sqrt{\gamma}^{t-i} \left\|\frac{\sqrt{1-\theta_i}g_i}{\sqrt{v_i}}\right\|^2\\
&\leq \frac{\alpha^2}{C_1\theta(1-\sqrt{\gamma})^2}\sum_{t=1}^T \left\|\frac{\sqrt{1-\theta_t}g_t}{\sqrt{v_t}}\right\|^2
\end{split}
\]
Thus, the desired result is obtained.
\end{proof}

\begin{lemma}\label{matrix}
By the iteration scheme of Algorithm 1, it holds that
\[
\sum_{t = 1}^T \|e_t\|\|\Delta_t\| \leq \sum_{t=1}^T\frac{1-\delta_g}{\delta_g} \|\Delta_t\|^2.
\]
\end{lemma}
\begin{proof}
By the definition of noisy term $e_{t}$ and $\Delta_{t}$, it holds
\[
\begin{split}
  \|e_t\|  &= \|\Delta_{t-1} + e_{t-1} - Q_g(\Delta_{t-1} + e_{t-1}) \| \leq (1-\delta_g) \|\Delta_{t-1} + e _{t-1}\|\leq (1-\delta_g) \|\Delta_{t-1}\| + (1-\delta_g)\|e_{t-1}\|\\
  &\leq \sum_{i=1}^{t-1} (1-\delta_g)^{t-i}\|\Delta_i\|.
\end{split}
\]
Therefore, we have 
\begin{align}\label{cross-noisy-eq}
    \sum_{t = 1}^T \|e_t\|\|\Delta_t\| \leq \sum_{t=1}^T\sum_{i=1}^{t-1} (1-\delta_g)^{t-i}\|\Delta_i\|\|\Delta_t\|.
\end{align}
In addition, let $\Delta = \left[ \begin{array}{cccc}\|\Delta_1\|&\|\Delta_2\|&\cdots&\|\Delta_T\|\end{array}\right]^{\top}$ and $U$ be the following $T\times T$ matrix:
\[
U = \left [ 
\begin{array}{ccccc}
0& (1-\delta_g)/2 & (1-\delta_g)^2/2 &\cdots&(1-\delta_g)^{T-1}/2\\
(1-\delta_g)/2 & 0& (1-\delta_g)/2 &\cdots&(1-\delta_g)^{T-2}/2\\
(1-\delta_g)^2/2 & (1-\delta_g)/2 & 0 &\cdots&(1-\delta_g)^{T-3}/2\\
\vdots&\vdots&\vdots&\ddots&\vdots\\
(1-\delta_g)^{T-1}/2 & (1-\delta_g)^{T-2}/2 & (1-\delta_g)^{T-3}/2 &\cdots&0
\end{array}\right].
\]
Let $\rho(U)$ be the spectral radius of $U$ and $\|U\|_{\infty}$ be $\infty$-norm which is defined to be the maximal row sum of $U$. Then, it holds that
\[
  \rho(U) \leq \|U\|_{\infty} \leq 2\sum_{t=1}^{T/2+1} (1-\delta_g)^t/2 \leq \frac{1-\delta_g}{\delta_g}.
\]
Utilizing the above inequality, we obtain 
\[
     \sum_{t=1}^T\sum_{i=1}^t (1-\delta_g)^{t-i+1}\|\Delta_i\|\|\Delta_t\| = \Delta^TU\Delta \leq \rho(U)\Delta^T\Delta \leq  \frac{1-\delta_g}{\delta_g} \sum_{t=1}^T\|\Delta_t\|^2.
\]
Substituting the above inequality into Eq.~\eqref{cross-noisy-eq}, we obtain the desired result.
\end{proof}

\begin{lemma}\label{sumgv}
The following estimate holds:
\[
\mathbb{E}\left[\sum_{t=1}^T\left\|\frac{\sqrt{1-\theta_t}g_t}{\sqrt{v_t}}\right\|^2\right] \leq d\left[\log\left(1+\frac{G^2}{\epsilon d}\right)+\frac{1}{1-\theta}\sum_{t=1}^T (1-\theta_t)\right].
\]
\end{lemma}

\begin{proof}
Let $W_0 = 1$ and $W_t = \prod_{i=1}^t \theta_i^{-1}$. Let $w_t = W_t-W_{t-1} = (1-\theta_t)W_t$. 

Therefore, we have $\frac{w_t}{W_t} = 1-\theta_t$, and $\frac{W_{t-1}}{W_t} = \theta_t$.

By observing that $W_0v_0 = \epsilon$ and $W_tv_t = W_{t-1}v_{t-1} + w_t g_t^2$, then we can obtain 
\[W_tv_t = \epsilon + \sum_{i=1}^tw_ig_i^2\].

By plugging the equality into the left hand side, we obtain
\[
\begin{split}
\sum_{t=1}^T\left\|\frac{\sqrt{1-\theta_t} g_t}{\sqrt{v_t}}\right\|^2 &= \sum_{t=1}^T \left\|\frac{(1-\theta_t)g_t^2}{v_t}\right\|_1 = \sum_{t=1}^T \left\|\frac{w_tg_t^2}{W_tv_t}\right\|_1 = \sum_{t=1}^T\left\|\frac{w_tg_t^2}{\epsilon + \sum_{i=1}^t w_ig_i^2}\right\|_1\\
& =\sum_{t=1}^T\sum_{k=1}^d \frac{w_tg_{t,k}^2}{\epsilon+\sum_{i=1}^t w_ig_{i,k}^2} = \sum_{k=1}^d\sum_{t=1}^T \frac{w_tg_{t,k}^2}{\epsilon+\sum_{i=1}^t w_ig_{i,k}^2}.
\end{split}
\] 

Considering each dimension respectively, for each $k=1,2,\cdots,d$, we obtain
\[
 \sum_{t=1}^T \frac{w_tg_{t,k}^2}{\epsilon+\sum_{i=1}^t w_ig_{i,k}^2} \leq \log\left(\epsilon + \sum_{i=1}^tw_ig_{i,k}^2\right) - \log(\epsilon) = \log\left(1 + \frac{1}{\epsilon}\sum_{i=1}^tw_ig_{i,k}^2\right).
\]

Therefore, 
\[
\begin{split}
\sum_{t=1}^T\left\|\frac{\sqrt{1-\theta_t} g_t}{\sqrt{v_t}}\right\|^2 &\leq \sum_{k=1}^d \log\left(1 + \frac{1}{\epsilon}\sum_{i=1}^Tw_ig_{i,k}^2\right) \leq  d\log\left(1 + \frac{1}{d\epsilon}\sum_{k=1}^d \sum_{i=1}^Tw_ig_{i,k}^2\right)\\
&= d\log\left(1 + \frac{1}{d\epsilon}\sum_{i=1}^Tw_i\|g_i\|^2\right) \leq d\log\left(1 + \frac{G^2}{d\epsilon}(W_T-W_0)\right)\\
&=d\log\left(1 + \frac{G^2}{d\epsilon}\left(\prod_{i=1}^T \theta_i^{-1} -1\right)\right) \leq d\left[\log\left(1+\frac{G^2}{d\epsilon}\right) + \sum_{t=1}^T\log(\theta_t^{-1})\right]\\
&\leq d\left[\log\left(1+\frac{G^2}{d\epsilon}\right) + \sum_{t=1}^T \left(\theta_t^{-1} -1\right)\right] \leq d\left[\log\left(1+\frac{G^2}{d\epsilon}\right) + \frac{1}{1-\theta}\sum_{t=1}^T (1-\theta_t)\right].
\end{split}
\]

Hence, we obtain desired result.
\end{proof}

\begin{lemma}\label{Mt}
By the definition of $M_t$, it holds that 
\[
\sum_{t=1}^T M_t \leq C_3d\alpha\left(\log\left(1+\frac{G^2}{\epsilon d}\right)+\frac{1}{1-\theta}\sum_{t=1}^T (1-\theta_t)\right)- \frac{1-\beta}{2}\sum_{t=1}^T\mathbb{E}\|\nabla f(x_t)\|_{\hat{\eta}_t}^2,
\]
where 
\[
\begin{split}
C_2 &= \left(\frac{\beta/(1-\beta)}{\sqrt{C_1(1-\gamma)\theta_1}}+1\right)^2\\
C_3 &= \frac{1}{\sqrt{C_1}(1-\sqrt{\gamma})} \left(\frac{\alpha L(2-\delta_g)}{C_1\theta(1-\sqrt{\gamma})^2\delta_g} + \frac{2C_2G}{\sqrt{\theta}} \right) 
\end{split}
\]
\end{lemma}
\begin{proof}
Using the definitions of $v_t$ and $\hat{v}_t$, we obtain
\[
\begin{split}
\frac{(1-\beta)\alpha_tg_t}{\sqrt{v_t}} &= \frac{(1-\beta)\alpha_tg_t}{\sqrt{\hat{v}_t}} + (1-\beta)\alpha_tg_t\left(\frac{1}{\sqrt{v_t}} - \frac{1}{\sqrt{\hat{v}_t}}\right)\\
&= (1-\beta)\hat{\eta}_tg_t + (1-\beta)\alpha_tg_t\frac{(1-\theta_t)(\sigma_t^2-g_t^2)}{\sqrt{v_t}\sqrt{\hat{v}_t}(\sqrt{v_t}+\sqrt{\hat{v}_t})}\\
&= (1-\beta)\hat{\eta}_tg_t+ \hat{\eta}_t\sigma_t\frac{(1-\theta_t)g_t}{\sqrt{v_t}}\frac{(1-\beta)\sigma_t}{\sqrt{v_t}+\sqrt{\hat{v}_t}} - \hat{\eta}_tg_t\frac{(1-\theta_t)g_t}{\sqrt{v_t}}\frac{(1-\beta)g_t}{\sqrt{v_t}+\sqrt{\hat{v}_t}}.
\end{split}
\]

In addition, we can obtain that
\[
\begin{split}
&\beta\alpha_tm_{t-1}\left(\frac{1}{\sqrt{v_t}} - \frac{1}{\sqrt{\theta_tv_{t-1}}}\right) = \beta\alpha_tm_{t-1}\frac{(1-\theta_t)g_t^2}{\sqrt{v_t}\sqrt{\theta_tv_{t-1}}(\sqrt{v_t}+\sqrt{\theta_tv_{t-1}})}\\
&\qquad =\beta\alpha_tm_{t-1}\frac{(1-\theta_t)g_t^2}{\sqrt{v_t}+\sqrt{\theta_tv_{t-1}}} + \beta\alpha_tm_{t-1} \frac{(1-\theta_t)g_t^2}{\sqrt{v_t}(\sqrt{v_t} + \sqrt{\theta_tv_{t-1}})} \left(\frac{1}{\sqrt{\theta_tv_{t-1}}} - \frac{1}{\sqrt{\hat{v}_t}}\right)\\
&\qquad = \hat{\eta}_tg_t\frac{(1-\theta_t)g_t}{\sqrt{v_t}}\left(\frac{\beta m_{t-1}}{\sqrt{v_t} +\sqrt{\theta_t v_{t-1}}}\right) + \frac{\beta\alpha_t m_{t-1}(1-\theta_t)g_t^2\sigma_t^2}{\sqrt{v_t}\sqrt{\hat{v}_t}\sqrt{\theta_tv_{t-1}}(\sqrt{v_t}+\sqrt{\theta_tv_{t-1}})(\sqrt{\hat{v}_t}+\sqrt{\theta_tv_{t-1}})}\\
& \qquad = \hat{\eta}_tg_t\frac{(1-\theta_t)g_t}{\sqrt{v_t}}\left(\frac{\beta m_{t-1}}{\sqrt{v_t} +\sqrt{\theta_t v_{t-1}}}\right) + \hat{\eta}_t\sigma_t\frac{(1-\theta_t)g_t}{\sqrt{v_t}}\left(\frac{\beta m_{t-1}}{\sqrt{\theta_tv_{t-1}}} \frac{\sqrt{1-\theta_t}g_t}{\sqrt{v_t}+\sqrt{\theta_tv_{t-1}}} \frac{\sqrt{1-\theta_t}\sigma_t}{\sqrt{\hat{v}_t}+\sqrt{\theta_tv_{t-1}}} \right).
\end{split}
\]

For convenience, we denote
\[
\begin{split}
A_t &= \frac{\beta m_{t-1}}{\sqrt{v_t} + \sqrt{\theta_t v_{t-1}}} - \frac{(1-\beta)g_t}{\sqrt{v_t} + \sqrt{\hat{v}_t}},\\
B_t &= \left(\frac{\beta m_{t-1}}{\sqrt{\theta_tv_{t-1}}} \frac{\sqrt{1-\theta_t}g_t}{\sqrt{v_t}+\sqrt{\theta_tv_{t-1}}} \frac{\sqrt{1-\theta_t}\sigma_t}{\sqrt{\hat{v}_t}+\sqrt{\theta_tv_{t-1}}} \right) +\frac{(1-\beta)\sigma_t}{\sqrt{v}_t +\sqrt{\hat{v}_t}}.
\end{split}
\]

Then, for each $t>2$, we obtain
\[
\begin{split}
\Delta_t - \frac{\beta\alpha_t}{\sqrt{\theta_t}\alpha_{t-1}}\Delta_{t-1} &= -\frac{\alpha_tm_t}{\sqrt{v_t}} + \frac{\beta\alpha_tm_{t-1}}{\sqrt{\theta_tv_{t-1}}} = -\alpha_t\left(\frac{m_t}{\sqrt{v_t}} - \frac{\beta m_{t-1}}{\sqrt{\theta_tv_{t-1}}}\right)\\
& = -\frac{(1-\beta)\alpha_tg_t}{\sqrt{v_t}} - \beta\alpha_tm_{t-1}\left(\frac{1}{\sqrt{v_t}} - \frac{1}{\sqrt{\theta_tv_{t-1}}}\right)\\
& = -(1-\beta)\hat{\eta}_tg_t - \hat{\eta}_tg_t\frac{(1-\theta_t)g_t}{\sqrt{v_t}}A_t - \hat{\eta}_t\sigma_t\frac{(1-\theta_t)g_t}{\sqrt{v_t}}B_t. 
\end{split}
\]

By using the above equality, we can get an upper bound for  $\mathbb{E}\langle \nabla f(x_t), \Delta_t\rangle$:
\[
\begin{split}
\mathbb{E} \langle \nabla f(x_t),\Delta_t \rangle &= \frac{\beta\alpha_t}{\sqrt{\theta_t}\alpha_{t-1}}\mathbb{E}\langle \nabla f(x_t),\Delta_{t-1}\rangle + \mathbb{E} \left\langle \nabla f(x_t),\Delta_t - \frac{\beta\alpha_t}{\sqrt{\theta_t}\alpha_{t-1}}\Delta_{t-1}\right\rangle\\
& = \frac{\beta\alpha_t}{\sqrt{\theta_t}\alpha_{t-1}}\mathbb{E}\langle \nabla f(x_t),\Delta_{t-1}\rangle - \mathbb{E} \left\langle \nabla f(x_t),(1-\beta)\hat{\eta}_tg_t\right\rangle \\
&\qquad - \mathbb{E}\left \langle \nabla f(x_t), \hat{\eta}_tg_t\frac{(1-\theta_t)g_t}{\sqrt{v_t}}A_t\right\rangle -\mathbb{E}\left\langle \nabla f(x_t), \hat{\eta}_t\sigma_t\frac{(1-\theta_t)g_t}{\sqrt{v_t}}B_t \right\rangle.
\end{split}
\]

We split $\mathbb{E}\langle \nabla f(x_t), \Delta_t\rangle$ into 4 terms, and we analyze these 4 terms respectively. For the first term, we obtain
\[
\begin{split}
\frac{\beta\alpha_t}{\sqrt{\theta_t}\alpha_{t-1}}\mathbb{E}\langle \nabla f(x_t),\Delta_{t-1}\rangle &= \frac{\beta\alpha_t}{\sqrt{\theta_t}\alpha_{t-1}}\mathbb{E}\left(\langle \nabla f(x_{t-1}), \Delta_{t-1}\rangle + \langle \nabla f(x_t) - \nabla f(x_{t-1}), \Delta_{t-1}\rangle \right)\\
&\leq \frac{\beta\alpha_t}{\sqrt{\theta_t}\alpha_{t-1}} \mathbb{E} (\langle \nabla f(x_{t-1}), \Delta_{t-1}\rangle + L\|x_t - x_{t-1}\|\|\Delta_{t-1}\|)\\
&\leq \frac{\beta\alpha_t}{\sqrt{\theta_t}\alpha_{t-1}} \mathbb{E} (\langle \nabla f(x_{t-1}), \Delta_{t-1}\rangle + L\|Q_g(\Delta_{t-1}+e_{t-1})\|\|\Delta_{t-1}\|)\\
&\leq \frac{\beta\alpha_t}{\sqrt{\theta_t}\alpha_{t-1}} \mathbb{E} (\langle \nabla f(x_{t-1}), \Delta_{t-1}\rangle\\ &\qquad + L\|Q_g(\Delta_{t-1}+e_{t-1}) - (\Delta_{t-1}+e_{t-1}) + (\Delta_{t-1}+e_{t-1})\|\|\Delta_{t-1}\|)\\
&\leq \frac{\beta\alpha_t}{\sqrt{\theta_t}\alpha_{t-1}} \mathbb{E} (\langle \nabla f(x_{t-1}), \Delta_{t-1}\rangle\\ &\qquad + L((1-\delta_g)\|\Delta_{t-1}+e_{t-1}\| + \|\Delta_{t-1}+e_{t-1}\|)\|\Delta_{t-1}\|)\\
&\leq \frac{\beta\alpha_t}{\sqrt{\theta_t}\alpha_{t-1}} \mathbb{E} (\langle \nabla f(x_{t-1}), \Delta_{t-1}\rangle + L(2-\delta_g)\|\Delta_{t-1}+e_{t-1}\|\|\Delta_{t-1}\|)\\
&\leq \frac{\beta\alpha_t}{\sqrt{\theta_t}\alpha_{t-1}} \mathbb{E} (\langle \nabla f(x_{t-1}), \Delta_{t-1}\rangle + L(2-\delta_g)\|\Delta_{t-1}\|^2+ L(2-\delta_g)\|e_{t-1}\|\|\Delta_{t-1}\|)\\
&= \frac{\beta\alpha_t}{\sqrt{\theta_t}\alpha_{t-1}} M_{t-1}.
\end{split}
\]

For the second term, we have
\[
-\mathbb{E}\langle\nabla f(x_t), (1-\beta)\hat{\eta}_tg_t\rangle = -(1-\beta) \mathbb{E}\langle \nabla f(x_t), \hat{\eta_t}\mathbb{E}_t(g_t)\rangle = -(1-\beta)\mathbb{E}\|\nabla f(x_t)\|_{\hat{\eta}_t}^2.
\]

For the third term, we have 
\[
\begin{split}
-\mathbb{E}\left\langle \nabla f(x_t), \hat{\eta}_tg_t \frac{(1-\theta_t)g_t}{\sqrt{v_t}} A_t \right\rangle &\leq \mathbb{E} \left\langle \frac{\sqrt{\hat{\eta}_t}|\nabla f(x_t)||g_t|}{\sigma_t}, \frac{\sqrt{\hat{\eta}_t}\sigma_t|A_t|(1-\theta_t)|g_t|}{\sqrt{v_t}}\right\rangle\\
&\leq \frac{1-\beta}{4}\mathbb{E}\left\|\frac{\sqrt{\hat{\eta}_t}|\nabla f(x_t)||g_t|}{\sigma_t}\right\|^2 + \frac{1}{1-\beta}\mathbb{E}\left\|\frac{\sqrt{\hat{\eta}_t}\sigma_t|A_t|(1-\theta_t)|g_t|}{\sqrt{v_t}}\right\|^2\\
&\leq \frac{1-\beta}{4}\mathbb{E}\|\nabla f(x_t)\|^2_{\hat{\eta}_t} + \frac{C_2G\alpha}{\theta}\mathbb{E}\left\|\frac{\sqrt{1-\theta_t}g_t}{\sqrt{v_t}}\right\|^2.
\end{split}
\]
where the inequality holds with the following equalities and inequalities:
\[
\mathbb{E}\left\|\frac{\sqrt{\hat{\eta}_t}|\nabla f(x_t)||g_t|}{\sigma_t}\right\|^2 = \mathbb{E}\left\|\frac{\hat{\eta}_t\nabla f(x_t)^2g_t^2}{\sigma_t^2}\right\|_1 = \mathbb{E} \|\hat{\eta}_t\nabla f(x_t)^2\|_1 = \mathbb{E}\|\nabla f(x_t)\|^2_{\hat{\eta}_t},
\]
\[
\sqrt{\hat{\eta}_t}\sigma_t \leq \sqrt{\frac{\alpha_t\sigma_t^2}{\sqrt{(1-\theta_t)\sigma_t^2}}} \leq \sqrt{\frac{\alpha G}{\sqrt{\theta}}},
\]
and 
\[
\begin{split}
|A_t| &\leq \frac{\beta|m_{t-1}|}{\sqrt{\theta_t v_{t-1}}} + \frac{(1-\beta)|g_t|}{\sqrt{v_t}} \leq  \frac{\beta}{\sqrt{\theta_tC_1(1-\gamma)(1-\theta_t)}} + \frac{1-\beta}{\sqrt{1-\theta_t}}.
\end{split}
\]

Let $C_2 = \left(\frac{\beta/(1-\beta)}{\sqrt{C_1(1-\gamma)\theta_1}}+1\right)^2$, we can obtain $|A_t|\leq \frac{\sqrt{C_2}(1-\beta)}{\sqrt{1-\theta_t}}$.

Then we obtain the upper bound of the third term.

For the fourth term, by using the similar inequalities we have
\[
|B_t| \leq \left(\frac{\beta|m_{t-1}|}{\sqrt{\theta_tv_{t-1}}} \frac{\sqrt{1-\theta_t}|g_t|}{\sqrt{v_t}+\sqrt{\theta_t v_t}}\frac{\sqrt{1-\theta_t}\sigma_t}{\sqrt{\hat{v}_t}+\sqrt{\theta_t v_{t-1}}}\right) + \frac{(1-\beta)\sigma_t}{\sqrt{v_t}+\sqrt{\hat{v}_t}} \leq \frac{(1-\beta)\sqrt{C_2}}{\sqrt{1-\theta_t}}.
\]

Then, the fourth term will be bounded as follows:
\[
\begin{split}
-\mathbb{E}\left\langle \nabla f(x_t), \hat{\eta}_t\sigma_t\frac{(1-\theta_t)g_t}{\sqrt{v_t}}B_t \right\rangle &\leq \mathbb{E}\left\langle \sqrt{\hat{\eta}}_t |\nabla f(x_t)|, \frac{\sqrt{\hat{\eta}_t}\sigma_t|B_t|(1-\theta_t)|g_t|}{\sqrt{v_t}}\right\rangle\\
&\leq \mathbb{E}\left\langle \sqrt{\hat{\eta}}_t |\nabla f(x_t)|, \frac{\frac{\sqrt{GC_2\alpha}}{\sqrt{\sqrt{\theta}}}\sqrt{1-\theta_t}|g_t|}{\sqrt{v_t}}\right\rangle\\
&\leq \frac{1-\beta}{4} \mathbb{E}\|\nabla f(x_t)\|_{\hat{\eta}_t}^2 + \frac{C_2G\alpha}{\sqrt{\theta}}\mathbb{E}\left\|\frac{\sqrt{1-\theta_t}g_t}{\sqrt{v_t}}\right\|^2
\end{split}
\]

Combining the above four terms, we obtain that
\[
\mathbb{E}\langle f(x_t),\Delta_t\rangle \leq \frac{\beta\alpha_t}{\sqrt{\theta_t}\alpha_{t-1}}M_{t-1} + \frac{2C_2G\alpha}{\sqrt{\theta}}\mathbb{E}\left\|\frac{\sqrt{1-\theta_t}g_t}{\sqrt{v_t}}\right\|^2 - \frac{1-\beta}{2}\mathbb{E}\|\nabla f(x_t)\|_{\hat{\eta}_t}^2
\]

On the other hand, Let $N_t = L(2-\delta_g)\mathbb{E}\|\Delta_t\|^2 + L(2-\delta_g)\mathbb{E}\|e_t\|\|\Delta_t\| + \frac{2C_2G\alpha}{\sqrt{\theta}}\mathbb{E}\left\|\frac{\sqrt{1-\theta_t}g_t}{\sqrt{v_t}}\right\|^2$, then with induction we can find the upper bound for $M_t$.  With the above bound, we have 
\[
M_t\leq \frac{\beta\alpha_t}{\sqrt{\theta_t}\alpha_{t-1}}M_{t-1}+ N_t - \frac{1-\beta}{2}\mathbb{E}\|\nabla f(x_t)\|_{\hat{\eta}_t}^2 \leq \frac{\beta\alpha_t}{\sqrt{\theta_t}\alpha_{t-1}}M_{t-1}+ N_t.
\] 

Besides, for $M_1$, we have
\[
\begin{split}
  M_1 &= \mathbb{E}\left\langle \nabla f(x_1), -\frac{\alpha_1 m_1}{\sqrt{v_1}}\right\rangle + L(2-\delta_g)\mathbb{E}\|\Delta_1\|^2 + L(2-\delta_g)\mathbb{E}\|e_1\|\|\Delta_1\|\\
  & = -\mathbb{E}\left\langle \nabla f(x_1), \frac{\alpha_1 (1-\beta)g_1}{\sqrt{v_1}}\right\rangle + L(2-\delta_g)\mathbb{E}\|\Delta_1\|^2 + L(2-\delta_g)\mathbb{E}\|e_1\|\|\Delta_1\|\\
  &= -\mathbb{E}\langle \nabla f(x_t), (1-\beta)\hat{\eta}_1g_1\rangle + \mathbb{E}\left\langle \nabla f(x_t), \hat{\eta}_1\sigma_1\frac{(1-\theta_1)g_1}{\sqrt{v_1}}\frac{(1-\beta)\sigma_1}{\sqrt{v_1}+\sqrt{\hat{v}_1}}\right\rangle \\
  & \qquad - \mathbb{E}\left\langle \nabla f(x_t), \hat{\eta}_1g_1\frac{(1-\theta_1)g_1}{\sqrt{v_1}}\frac{(1-\beta)g_1}{\sqrt{v_1}+\sqrt{\hat{v}_1}} \right\rangle + L(2-\delta_g)\mathbb{E}\|\Delta_1\|^2 + L(2-\delta_g)\mathbb{E}\|e_1\|\|\Delta_1\|\\
  &\leq \frac{2C_2G\alpha}{\sqrt{\theta}}\mathbb{E}\left\|\frac{\sqrt{1-\theta_1}g_1}{\sqrt{v_1}}\right\|^2 - \frac{1-\beta}{2}\mathbb{E}\|\nabla f(x_t)\|_{\hat{\eta}_t}^2 + L(2-\delta_g)\mathbb{E}\|\Delta_1\|^2 + L(2-\delta_g)\mathbb{E}\|e_1\|\|\Delta_1\|\\
  &\leq N_1. 
  \end{split}
\]

Therefore, we can obtain
\[
\begin{split}
M_t \leq \sum_{i=1}^t \frac{\alpha_t\beta^{t-i}}{\alpha_i\sqrt{\Theta(t,i)}}N_i - \frac{1-\beta}{2}\mathbb{E}\|\nabla f(x_t)\|_{\hat{\eta}_t}^2 \leq \frac{1}{\sqrt{C_1}} \sum_{i=1}^t \sqrt{\gamma}^{t-i}N_i - \frac{1-\beta}{2}\mathbb{E}\|\nabla f(x_t)\|_{\hat{\eta}_t}^2,
\end{split}
\]
where the last inequality is because $\alpha_t\leq \alpha_i$ and $\Theta(t,i)\geq C_1 (\theta')^{t-i}$.

Then, by summing $M_t$ up, we obtain
\[
\begin{split}
\sum_{t=1}^T M_t &\leq \frac{1}{\sqrt{C_1}}\sum_{t=1}^T\sum_{i=1}^t\sqrt{\gamma}^{t-i} N_i - \frac{1-\beta}{2}\sum_{t=1}^T\mathbb{E}\|\nabla f(x_t)\|_{\hat{\eta}_t}^2\\
& = \frac{1}{\sqrt{C_1}}\sum_{i=1}^T\sum_{t=i}^T\sqrt{\gamma}^{t-i} N_i - \frac{1-\beta}{2}\sum_{t=1}^T\mathbb{E}\|\nabla f(x_t)\|_{\hat{\eta}_t}^2\\
&\leq \frac{1}{\sqrt{C_1}(1-\sqrt{\gamma})}\sum_{t=1}^T N_t - \frac{1-\beta}{2}\sum_{t=1}^T\mathbb{E}\|\nabla f(x_t)\|_{\hat{\eta}_t}^2.
\end{split}
\]

Meanwhile, we can bound summation of $N_t$ by the following terms:
\[
\begin{split}
\sum_{t=1}^T N_t &= \sum_{t=1}^T L(2-\delta_g)\mathbb{E}\|\Delta_t\|^2 + L(2-\delta_g)\mathbb{E}\|e_t\|\|\Delta_t\| + \frac{2C_2G\alpha}{\sqrt{\theta}}\mathbb{E}\left\|\frac{\sqrt{1-\theta_t}g_t}{\sqrt{v_t}}\right\|^2\\
&\leq \sum_{t=1}^T \frac{L(2-\delta_g)}{\delta_g}\mathbb{E}\|\Delta_t\|^2 + \frac{2C_2G\alpha}{\sqrt{\theta}}\mathbb{E}\left\|\frac{\sqrt{1-\theta_t}g_t}{\sqrt{v_t}}\right\|^2\\
&\leq \sum_{t=1}^T\left(\frac{\alpha^2L(2-\delta_g)}{C_1\theta(1-\sqrt{\gamma})^2\delta_g} + \frac{2C_2G\alpha}{\sqrt{\theta}} \right)\mathbb{E}\left\|\frac{\sqrt{1-\theta_t}g_t}{\sqrt{v_t}}\right\|^2\\
&\leq \left(\frac{\alpha^2L(2-\delta_g)}{C_1\theta(1-\sqrt{\gamma})^2\delta_g} + \frac{2C_2G\alpha}{\sqrt{\theta}} \right) d\left[\log\left(1+\frac{G^2}{\epsilon d}\right)+\frac{1}{1-\theta}\sum_{t=1}^T (1-\theta_t)\right].
\end{split}
\]
Thus, by combining those inequalities we obtain the desired result.
\end{proof}

\begin{proof}[Proof of Theorem 1]
 Based on Notation \eqref{notation-thm1} and the above lemmas, then we can prove Theorem 1. First, according to the gradient Lipschitz condition of $f$, it holds
\[
\begin{split}
f(\tilde{x}_{t+1}) &\leq f(\tilde{x}_t) + \langle\nabla f(\tilde{x}_t), \Delta_t\rangle + \frac{L}{2} \|\Delta_t^2\|\\
& =  f(\tilde{x}_t) + \langle\nabla f(x_t), \Delta_t\rangle + \frac{L}{2} \|\Delta_t\|^2 +\langle\nabla f(\tilde{x}_t)  - \nabla f(x_t), \Delta_t\rangle\\
&\leq  f(\tilde{x}_t) + \langle\nabla f(x_t), \Delta_t\rangle + \frac{L}{2} \|\Delta_t\|^2 + \|\nabla f(\tilde{x}_t) - \nabla f(x_t)\|\|\Delta_t\|\\
&\leq f(\tilde{x}_t) + \langle\nabla f(x_t), \Delta_t\rangle +  L(2-\delta_g)\|\Delta_t\|^2 + L(2-\delta_g)\|e_t\|\|\Delta_t\|.
\end{split}
\]
Recall that $M_t = \mathbb{E}[\langle\nabla f(x_t), \Delta_t\rangle+L(2-\delta_g)\|\Delta_t\|^2 + L(2-\delta_g)\|e_t\|\|\Delta_t\|]$. 
Then we have
\[
\begin{split}
    f^*&\leq \mathbb{E}[f(\tilde{x}_{T+1})] \leq f(x_1) + \sum_{t=1}^T M_t\\
    & \leq f(x_1) + \sum_{t=1}^T M_t\leq f(x_1) + C_3d\alpha\left(\log\left(1+\frac{G^2}{\epsilon d}\right)+\frac{1}{1-\theta}\sum_{t=1}^T (1-\theta_t)\right)- \frac{1-\beta}{2}\sum_{t=1}^T\mathbb{E}\|\nabla f(x_t)\|_{\hat{\eta}_t}^2.\\
\end{split}
\]
Using the above lemmas and arranging the corresponding terms, we have
\[
\begin{split}
    (\mathbb{E}[\|\nabla f((x_\tau^T))\|^2]) &\leq \frac{\sqrt{G^2+\epsilon d}}{\alpha\sqrt{T}}\mathbb{E}\left[\sum_{t=1}^T\|\nabla f(x_t)\|_{\hat{\eta}_t}^2\right]\\&\leq \frac{2\sqrt{G^2+\epsilon d}}{(1-\beta)\alpha\sqrt{T}}\left(f(x_1) - f^* + C_3d\alpha\left(\log\left(1+\frac{G^2}{\epsilon d}\right)+\frac{1}{1-\theta}\sum_{t=1}^T (1-\theta_t)\right)\right)\\
    & \leq \frac{C+C'\sum_{t=1}^T\frac{1}{t}}{\sqrt{T}},
\end{split}
\]
where $C_3$, $C'$ and $C'$ are defined as follows,
\[
\begin{split}
    C_2 &= \left(\frac{\beta/(1-\beta)}{\sqrt{C_1(1-\gamma)\theta_1}}+1\right)^2,\\
    C_3 &= \frac{1}{\sqrt{C_1}(1-\sqrt{\gamma})} \left(\frac{\alpha L(2-\delta_g)}{C_1\theta(1-\sqrt{\gamma})^2\delta_g} + \frac{2C_2G}{\sqrt{\theta}} \right),\\ 
    C &= \frac{2\sqrt{G^2+\epsilon d}}{(1-\beta)\alpha}\left(f(x_1)-f^*+ \alpha C_3d\log\left(1+\frac{G^2}{\epsilon d}\right)\right),\\
    C'& = \frac{2\sqrt{G^2+\epsilon d}C_3d}{(1-\beta)(1-\theta)},
\end{split}
\]
respectively. Hence, the proof is completed.
\end{proof}

\subsection{Proof of Theorem 2}\label{pft2}
To prove Theorem 2, we still need some useful lemmas and notations as follows:
\begin{notation}\label{notation-thm2}
Let $\mathbb{E}_t(\cdot) = \mathbb{E}_\xi(\cdot|x_t)$. 
Denote 
${\sigma^{(i)}_t}^2 = \mathbb{E}_t(g_t^2)$, 
$\hat{v}^{(i)}_t = \theta_t v^{(i)}_t + (1-\theta_t) {\sigma^{(i)}}^2_t$, 
$\hat{\eta}^{(i)}_t = \alpha_t/\sqrt{\hat{\theta}^{(i)}_t}$, 
$\Delta_t^{(i)} = -\alpha_t m_t^{(i)}/\sqrt{v_t^{(i)}}$,
$\Delta_t = \frac{1}{N}\sum_{i=1}^N \Delta_t^{(i)}$, 
$E_t = \frac{1}{N}\sum_{i=1}^N e_t^{(i)}$, and,
$M_t = \mathbb{E}[\langle \nabla f(x_{t}),\Delta_{t}\rangle + \frac{L(2-\delta_x)}{N}\sum_{i=1}^N \|e_{t}\|\|\Delta_{t}^{(i)}\| + \frac{L(2-\delta_x)(2-\delta_g)}{N}\sum_{i=1}^N \|\Delta_{t}^{(i)}\|^2 $ $+ \frac{L(2-\delta_x)(2-\delta_g)}{N^2}\sum_{i=1}^N\sum_{j=1}^N\|e_{t}^{(i)}\|\|\Delta_{t}^{(j)}\|]$.

In addition, let $\tilde{x}_t = x_t - e_{t}$, and,  $ \hat{x_t} = \tilde{x}_t - E_t$. 

Then, it holds that  $\tilde{x}_{t+1} = x_t - Q_x(\hat{\delta}_t+e_t) - e_{t+1} = x_t + \hat{\delta}_t -e_t = \tilde{x}_t + \hat{\delta}_t$.

Besides, $\hat{x}_{t+1} = \tilde{x_t} - \frac{1}{N}\sum_{t=1}^N Q_g(-\Delta_t^{(i)} +e_t^{(i)}) - E_{t+1} = \tilde{x_t} - \frac{1}{N}\sum_{t=1}^N -\Delta_t^{(i)} - E_{t} = \hat{x}_t + \Delta_t$.
\end{notation}

\begin{lemma}
Let $e^{(i)}_t$ be the noisy term defined in Algorithm \ref{alg2} and $\Delta^{(i)}_t$ be the term defined in Notation \ref{notation-thm2}. Then it holds that 
\[
\mathbb{E}\left[\frac{1}{N^2}\sum_{t=1}^T\sum_{i=1}^N\sum_{j=1}^N \|e_t^{(i)}\|\|\Delta_t^{(j)}\|\right] \leq \frac{1-\delta_g}{\delta_gN}\sum_{i=1}^N \mathbb{E}\left[\sum_{t=1}^T\|\Delta_t^{(i)}\|^2\right].
\]
\end{lemma}
\begin{proof}
Using the definition of the noisy term  $e_{t}$, the following holds:
\[
    \|e^{(j)}_t\| = \|\Delta_{t-1}^{(j)} + e_{t-1}^{(j)} - Q_g(\Delta_{t-1}^{(j)} + e_{t-1}^{(j)})\| \leq (1-\delta_g) (\|\Delta_{t-1}^{(j)}\| + \|e_{t-1}^{(j)}\|) \leq \sum_{k = 1}^{t-1} (1-\delta_g)^{t-k} \|\Delta_k^{(j)}\|.
\]

When $t_1<t_2$, it holds that:
\begin{align*}
    E(\Delta_{t_1}^{(i)}\Delta_{t_2}^{(j)}) &= E(E(\Delta_{t_1}^{(i)}\Delta_{t_2}^{(j)}|x_{t_2}))= E(E(\Delta_{t_1}^{(i)}|x_{t_2})E(\Delta_{t_2}^{(j)}|x_{t_2})) \\
&= E(E(\Delta_{t_1}^{(i)}|x_{t_2})E(\Delta_{t_2}^{(i)}|x_{t_2})) =E(E(\Delta_{t_1}^{(i)}\Delta_{t_2}^{(i)})|x_{t_2})\\
&=E(\Delta_{t_1}^{(i)}\Delta_{t_2}^{(i)}),
\end{align*}
where the equalities hold since worker i and worker j work in the same setting and independently.
%
%On the other hand, when $t_1=t_2, i\neq j$, since workers $i$ and $j$ work independently, it holds that
%\begin{align*}
%    E(\Delta_{t_1}^{(i)}\Delta_{t_2}^{(j)}) 
%&= E(\Delta_{t_1}^{(i)})E(\Delta_{t_2}^{(j)}) = E(\Delta_{t_1}^{(i)})^2 \leq E([\Delta_{t_1}^{(i)}]^2).
%\end{align*} 

Then, we have 
\[
\begin{split}
\mathbb{E}\left[\frac{1}{N^2}\sum_{t=1}^T\sum_{i=1}^N\sum_{j=1}^N \|e_t^{(i)}\|\|\Delta_t^{(j)}\|\right] &\leq
\mathbb{E}\left[\frac{1}{N^2}\sum_{t=1}^T\sum_{i=1}^N\sum_{j=1}^N\sum_{k=1}^{t-1} (1-\delta_g)^{t-k}\|\Delta_k^{(i)}\|\|\Delta_t^{(j)}\|\right]\\
&\leq \mathbb{E}\left[\frac{1}{N}\sum_{t=1}^T\sum_{k=1}^{t-1}\sum_{i=1}^N(1-\delta_g)^{t-k} \|\Delta_k^{(i)}\|\|\Delta_t^{(i)}\|\right]\\
&\leq \frac{1-\delta_g}{\delta_gN}\sum_{t=1}^T\sum_{i=1}^N \mathbb{E}\|\Delta_t^{(i)}\|^2,
\end{split}
\]
where the last inequality can be proven by Lemma \ref{matrix}. Hence, the proof is completed.
\end{proof}

\begin{lemma}
Let $e_t$ be the noisy term defined in Algorithm \ref{alg1} and $\Delta^{(i)}_t$ be the term defined in Notation \ref{notation-thm2}. Then it holds that 
\[
\mathbb{E}\left[\frac{1}{N}\sum_{t=1}^T\sum_{i=1}^N\|e_t\|\|\Delta_t^{(i)}\|\right] \leq \frac{(1-\delta_x)(2-\delta_g)}{N\delta_x\delta_g}\sum_{i=1}^N \mathbb{E}\left[\sum_{t=1}^T\|\Delta_t^{(i)}\|^2\right]
\]
\end{lemma}
\begin{proof}
With the definition of $e_t$, we obtain
\[
\begin{split}
\|e_t\| &= \|\hat{\delta}_{t-1} + e_{t-1} - Q_x(\hat{\delta}_{t-1} + e_{t-1})\| \leq (1-\delta_x)(\|\hat{\delta}_{t-1}\| + \|e_{t-1}\|)\\
 &=(1-\delta_x)\left(\frac{1}{N}\left\|\sum_{j = 1}^N Q_g(\Delta_{t-1}^{(j)} + e_{t-1}^{(j)})\right\| + \|e_{t-1}\|\right)\\ 
 &\leq (1-\delta_x)\left(\frac{1}{N}\left\|\sum_{j = 1}^N Q_g(\Delta_{t-1}^{(j)} + e_{t-1}^{(j)}) - \Delta_{t-1}^{(j)} + e_{t-1}^{(j)}\right\| +\frac{1}{N}\sum_{j=1}^N\|\Delta_{t-1}^{(j)} + e_{t-1}^{(j)}\| + \|e_{t-1}\|\right)\\
 &\leq (1-\delta_x)\left(\frac{2-\delta_g}{N}\sum_{j=1}^N\|\Delta_{t-1}^{(j)}\| + \frac{2-\delta_g}{N}\sum_{j=1}^N\|e_{t-1}^{(j)}\| + \|e_{t-1}\|\right) \\
&\leq \frac{1}{N}(1-\delta_x)((2-\delta_g)\sum_{j=1}^N\|\Delta_{t-1}^{(j)}\| + (2-\delta_g)\sum_{j=1}^N\sum_{k=1}^{t-1}(1-\delta_g)^{t-k}\|\Delta_k^{(j)}\| + \|e_{t-1}\|)\\
&\leq \frac{1}{N}\sum_{l=1}^{t-1} (1-\delta_x)^{t-l}(2-\delta_g)(\sum_{j=1}^N\|\Delta_l^{(j)}\| + \sum_{j=1}^N\sum_{k = 1}^{l-1} (1-\delta_g)^{l-k}\|\Delta_k^{(j)}\|)
\end{split} 
\]

Besides, for sequence $\{a_i\}$, we have
\[
\begin{split}
\sum_{t=1}^T\sum_{l=1}^{t-1}\sum_{k=1}^{l-1} (1-\delta_x)^{t-l}(1-\delta_g)^{l-k}a_ka_t &= \sum_{t=1}^T\sum_{k=1}^{t-1}\sum_{l=k+1}^{t-1} (1-\delta_x)^{t-l}(1-\delta_g)^{l-k}a_ka_t\\
\end{split}
\]

By similar construction of matrix in Lemma \ref{matrix}, we get the matrix U, where
$U_{i,j} = \frac{1}{2}\sum_{l=min(i,j)+1}^{max(i,j)-1}(1-\delta_x)^{max(i,j)-l}(1-\delta_g)^{l-min(i,j)}$ for $i\neq j$, and $U_{i,i} = 0$.

Therefore $U_{\infty}\leq 2*\frac{1}{2} \sum_{t=1}^T \sum_{l=t+1}^{T-1} (1-\delta_x)^{T-l} (1-\delta_g)^{l-t}\leq \frac{(1-\delta_x)(1-\delta_g)}{\delta_x\delta_g}$. 

So, we can get $\sum_{t=1}^T\sum_{l=1}^{t-1}\sum_{k=1}^{l-1} (1-\delta_x)^{t-l}(1-\delta_g)^{l-k}a_ka_t \leq  \frac{(1-\delta_x)(1-\delta_g)}{\delta_x\delta_g}\sum_{t=1}^T a_t^2$.

Because each worker works independently, by substituting the result in, we have
\[
\begin{split}
&\mathbb{E}\left[\frac{1}{N}\sum_{t=1}^T\sum_{i=1}^N\|e_t\|\|\Delta_t^{(i)}\|\right] \\
&\leq \mathbb{E}\left[\frac{1}{N^2}\sum_{t=1}^T\sum_{i=1}^N\sum_{l=1}^{t-1}\sum_{j=1}^N(1-\delta_x)^{t-l}(2-\delta_g)\left(\|\Delta_l^{(j)}\||\Delta_t^{(i)}\| + \sum_{k=1}^{l-1}(1-\delta_g)^{l-k}\|\Delta_k^{(j)}\|\|\Delta_t^{(i)}\|\right)\right]\\
&\leq \mathbb{E}\left[\frac{1}{N} \sum_{t=1}^T\sum_{i=1}^N\sum_{l=1}^{t-1} (1-\delta_x)^{t-l}(2-\delta_g)\left(\|\Delta_l^{(i)}\|\|\Delta_t^{(i)}\| + \sum_{k=1}^{l-1}(1-\delta_g)^{l-k}\|\Delta_k^{(i)}\|\|\Delta_t^{(i)}\|\right)\right]\\
&\leq \mathbb{E}\left[\frac{(1-\delta_x)(2-\delta_g)}{N\delta_x}\sum_{t=1}^T\sum_{i=1}^N\|\Delta_t^{(i)}\|^2 + \frac{(1-\delta_x)(1-\delta_g)(2-\delta_g)}{N\delta_x\delta_g}\sum_{t=1}^T\sum_{i=1}^N\|\Delta_t^{(i)}\|^2\right]\\
& = \mathbb{E}\left[\frac{(1-\delta_x)(2-\delta_g)}{N\delta_x\delta_g}\sum_{t=1}^T\sum_{i=1}^N\|\Delta_t^{(i)}\|^2\right]
\end{split}
\]
\end{proof}

\begin{lemma}\label{Mtmul}
By the definition of $M_t$, it holds that 
\[
\sum_{t=1}^T M_t \leq C_4d\alpha\left(\log\left(1+\frac{G^2}{\epsilon d}\right)+\frac{1}{1-\theta}\sum_{t=1}^T (1-\theta_t)\right)- \frac{1-\beta}{2N}\sum_{i=1}^N\sum_{t=1}^T\mathbb{E}\|\nabla f(x_t)\|_{\hat{\eta}_t^{(i)}}^2,
\]
where 
\[
\begin{split}
C_2 &= \left(\frac{\beta/(1-\beta)}{\sqrt{C_1(1-\gamma)\theta_1}}+1\right)^2\\
C_4 &= \frac{1}{\sqrt{C_1}(1-\sqrt{\gamma})} \left(\frac{\alpha L(2-\delta_x)(2-\delta_g)}{C_1\theta(1-\sqrt{\gamma})^2\delta_x\delta_g} + \frac{2C_2G}{\sqrt{\theta}}\right)
\end{split}
\]
\end{lemma}
\begin{proof}
Similar to Lemma \ref{Mt}, we define $A_t^{(i)}$ and $B_t^{(i)}$ as follows:
\[
\begin{split}
A_t^{(i)} &= \frac{\beta m_{t-1}^{(i)}}{\sqrt{v_t^{(i)}}+\sqrt{\theta_tv_{t-1}^{(i)}}} - \frac{(1-\beta)g_t^{(i)}}{\sqrt{v_t^{(i)}}+\sqrt{\hat{v}_t^{(i)}}},\\
B_t^{(i)} &= \left(\frac{\beta m_{t-1}^{(i)}}{\sqrt{\theta_t v_{t-1}^{(i)}}} \frac{\sqrt{1-\theta_t}g_t^{(i)}}{\sqrt{v_t^{(i)}} +\sqrt{\theta_tv_{t-1}^{(i)}}}\frac{(1-\theta_t)\sigma_t^{(i)}}{\sqrt{\hat{v}_t^{(i)}} + \sqrt{\theta_tv_{t-1}^{(i)}}}\right) + \frac{(1-\beta)\sigma_t^{(i)}}{\sqrt{v_t^{(i)}}+\sqrt{\hat{v}_t^{(i)}}}.
\end{split}
\]

Still,  we can split $\mathbb{E}\langle \nabla f(x_t),\Delta_t\rangle$ into four terms:
\[
\begin{split}
\mathbb{E}\langle \nabla f(x_t),\Delta_t\rangle &= \frac{\beta\alpha_t}{\sqrt{\theta_t}\alpha_{t-1}}\mathbb{E}\langle \nabla f(x_t),\Delta_{t-1}\rangle - \frac{1}{N}\sum_{i=1}^N \mathbb{E}\langle \nabla f(x_t), (1-\beta)\hat{\eta}_t^{(i)} g_t^{(i)}\rangle \\
& \qquad - \frac{1}{N}\sum_{i=1}^N\mathbb{E}\left\langle \nabla f(x_t), \hat{\eta}_t^{(i)}g_t^{(i)}\frac{(1-\theta_t)g_t^{(i)}}{\sqrt{v_t^{(i)}}}A_t^{(i)} \right\rangle\\ &\qquad- \frac{1}{N} \sum_{i=1}^N \mathbb{E}\left \langle \nabla f(x_t), \hat{\eta}_t^{(i)}\sigma_t^{(i)}\frac{(1-\theta_t)g_i^{(i)}}{\sqrt{v_t^{(i)}}}B_t^{(i)}\right\rangle 
\end{split}
\]

For the first term, we obtain
\[
\begin{split}
\mathbb{E}\langle \nabla f(x_t),\Delta_{t-1}\rangle  &= \mathbb{E}\langle \nabla f(x_{t-1}),\Delta_{t-1}\rangle + \mathbb{E}\langle \nabla f(x_t)-\nabla f(x_{t-1}),\Delta_{t-1}\rangle\\
&\leq \mathbb{E}\langle \nabla f(x_{t-1}),\Delta_{t-1}\rangle + \mathbb{E} \|\nabla f(x_t)-\nabla f(x_{t-1})\|\|\Delta_{t-1}\|\\
&\leq \mathbb{E}\langle \nabla f(x_{t-1}),\Delta_{t-1}\rangle + L\mathbb{E} \left\|Q_x\left(\frac{1}{N}\sum_{i=1}^N Q_g(\Delta_{t-1}^{(i)}+e_{t-1}^{(i)}) +e_{t-1}\right)\right\|\|\Delta_{t-1}\|\\
&\leq \mathbb{E}\langle \nabla f(x_{t-1}),\Delta_{t-1}\rangle + L(2-\delta_x)\mathbb{E} \left\|\frac{1}{N}\sum_{i=1}^N Q_g(\Delta_{t-1}^{(i)}+e_{t-1}^{(i)}) +e_{t-1}\right\|\|\Delta_{t-1}\|\\
&\leq \mathbb{E}\langle \nabla f(x_{t-1}),\Delta_{t-1}\rangle + L(2-\delta_x)\mathbb{E}\|e_{t-1}\|\|\Delta_{t-1}\|\\&\qquad + L(2-\delta_x)(2-\delta_g) \frac{1}{N}\sum_{i=1}^N \|\Delta_{t-1}^{(i)}\|\|\Delta_{t-1}\|+ L(2-\delta_x)(2-\delta_g)\mathbb{E}\frac{1}{N}\sum_{i=1}^N\|e_{t-1}^{(i)}\|\|\Delta_{t-1}\|\\
&\leq \mathbb{E}\langle \nabla f(x_{t-1}),\Delta_{t-1}\rangle + \frac{L(2-\delta_x)}{N}\sum_{i=1}^N \mathbb{E}\|e_{t-1}\|\|\Delta_{t-1}^{(i)}\|
\\&\qquad +  \frac{L(2-\delta_x)(2-\delta_g)}{N}\sum_{i=1}^N \mathbb{E}\|\Delta_{t-1}^{(i)}\|^2+ \frac{L(2-\delta_x)(2-\delta_g)}{N^2}\mathbb{E}\sum_{i=1}^N\sum_{j=1}^N\|e_{t-1}^{(i)}\|\|\Delta_{t-1}^{(j)}\|\\
&=M_{t-1}.
\end{split}
\]

The second term remain the same as it is in the lemma \ref{Mt}, in which we obtain
\[
-\frac{1}{N}\sum_{i=1}^N\mathbb{E}\langle \nabla f(x_t),(1-\beta)\hat{\eta}_t^{(i)}g_t^{(i)}\rangle = -\frac{1-\beta}{N}\sum_{i=1}^N \|\nabla f(x_t)\|_{\hat{\eta}_t^{(i)}}^2.
\]

The third term can have similar derivation as it is in the lemma \ref{Mt}, we obtain
\[
-\frac{1}{N}\mathbb{E}\sum_{i=1}^N\left\langle \nabla f(x_t), \hat{\eta}_t^{(i)}g_t^{(i)}\frac{(1-\theta_t)g_t^{(i)}}{\sqrt{v_t^{(i)}}}A_t\right\rangle \leq \frac{1}{N}\sum_{i=1}^N \frac{1-\beta}{4}\mathbb{E}\|\nabla f(x_t)\|_{\hat{\eta}_t^{(i)}}^2 + \frac{C_2G\alpha}{\sqrt{\theta}}\mathbb{E}\left\|\frac{\sqrt{1-\theta_t}g_t^{(i)}}{\sqrt{v_t^{(i)}}}\right\|^2.
\]

And for the fourth term, we have
\[
- \frac{1}{N} \sum_{i=1}^N \mathbb{E}\left \langle \nabla f(x_t), \hat{\eta}_t^{(i)}\sigma_t^{(i)}\frac{(1-\theta_t)g_i^{(i)}}{\sqrt{v_t^{(i)}}}B_t^{(i)}\right\rangle \leq \frac{1}{N}\sum_{i=1}^N \frac{1-\beta}{4}\mathbb{E}\|\nabla f(x_t)\|_{\hat{\eta}_t^{(i)}}^2 + \frac{C_2G\alpha}{\sqrt{\theta}}\mathbb{E}\left\|\frac{\sqrt{1-\theta_t}g_t^{(i)}}{\sqrt{v_t^{(i)}}}\right\|^2.
\] 

By defining $N_t =  \frac{L(2-\delta_x)}{N}\sum_{i=1}^N \mathbb{E}\|e_{t}\|\|\Delta_{t}^{(i)}\|
+  \frac{L(2-\delta_x)(2-\delta_g)}{N}\sum_{i=1}^N \mathbb{E}\|\Delta_{t}^{(i)}\|^2+ \frac{L(2-\delta_x)(2-\delta_g)}{N^2}\mathbb{E}\sum_{i=1}^N\sum_{j=1}^N\|e_{t}^{(i)}\|\|\Delta_{t}^{(j)}\| + \frac{1}{N}\sum_{i=1}^N \frac{2C_2G\alpha}{\sqrt{\theta}}\mathbb{E}\left\|\frac{\sqrt{1-\theta_t}g_t^{(i)}}{\sqrt{v_t^{(i)}}}\right\|^2$, then with the same induction in Lemma \ref{Mt}, we obtain
\[
\begin{split}
\sum_{t=1}^T M_t \leq \frac{1}{\sqrt{C_1}(1-\sqrt{\gamma})}\sum_{t=1}^T N_t - \frac{1-\beta}{2N}\sum_{i=1}^N\sum_{t=1}^T\mathbb{E}\|\nabla f(x_t)\|_{\hat{\eta}_t^{(i)}}^2.
\end{split}
\]

Besides, we have
\[
\begin{split}
\sum_{t=1}^T N_t &= \sum_{t=1}^T \frac{L(2-\delta_x)}{N}\sum_{i=1}^N \mathbb{E}\|e_{t}\|\|\Delta_{t}^{(i)}\|
+  \frac{L(2-\delta_x)(2-\delta_g)}{N}\sum_{i=1}^N \mathbb{E}\|\Delta_{t}^{(i)}\|^2 \\&\qquad + \frac{L(2-\delta_x)(2-\delta_g)}{N^2}\mathbb{E}\sum_{i=1}^N\sum_{j=1}^N\|e_{t}^{(i)}\|\|\Delta_{t}^{(j)}\| + \frac{1}{N}\sum_{i=1}^N \frac{2C_2G\alpha}{\sqrt{\theta}}\mathbb{E}\left\|\frac{\sqrt{1-\theta_t}g_t^{(i)}}{\sqrt{v_t^{(i)}}}\right\|^2\\
&\leq \frac{L(2-\delta_x)(1-\delta_x)(2-\delta_g)}{N\delta_x\delta_g}\sum_{i=1}^N \sum_{t=1}^T \mathbb{E} \|\Delta_t^{(i)}\|^2 + \frac{L(2-\delta_x)(2-\delta_g)}{N}\sum_{t=1}^T\sum_{i=1}^N \mathbb{E}\|\Delta_{t}^{(i)}\|^2\\ &\qquad +\frac{L(2-\delta_x)(2-\delta_g)(1-\delta_g)}{\delta_gN}\sum_{i=1}^N \sum_{t=1}^T\mathbb{E}\|\Delta_t^{(i)}\|^2 +  \frac{1}{N}\sum_{i=1}^N \sum_{t=1}^T\frac{2C_2G\alpha}{\sqrt{\theta}}\mathbb{E}\left\|\frac{\sqrt{1-\theta_t}g_t^{(i)}}{\sqrt{v_t^{(i)}}}\right\|^2\\
& = \frac{L(2-\delta_x)(2-\delta_g)}{N\delta_x\delta_g}\sum_{i=1}^N \sum_{t=1}^T \mathbb{E} \|\Delta_t^{(i)}\|^2 +\frac{1}{N}\sum_{i=1}^N \sum_{t=1}^T\frac{2C_2G\alpha}{\sqrt{\theta}}\mathbb{E}\left\|\frac{\sqrt{1-\theta_t}g_t^{(i)}}{\sqrt{v_t^{(i)}}}\right\|^2\\
&\leq \left(\frac{\alpha^2L(2-\delta_x)(2-\delta_g)}{C_1\theta(1-\sqrt{\gamma})^2\delta_x\delta_g} + \frac{2C_2G\alpha}{\sqrt{\theta}}\right) \frac{1}{N} \sum_{i=1}^N \sum_{t=1}^T\mathbb{E}\left\|\frac{\sqrt{1-\theta_t}g_t^{(i)}}{\sqrt{v_t^{(i)}}}\right\|^2\\
&\leq  \left(\frac{\alpha^2L(2-\delta_x)(2-\delta_g)}{C_1\theta(1-\sqrt{\gamma})^2\delta_x\delta_g} + \frac{2C_2G\alpha}{\sqrt{\theta}}\right) d\left[\log\left(1+\frac{G^2}{\epsilon d}\right)+\frac{1}{1-\theta}\sum_{t=1}^T (1-\theta_t)\right]
\end{split}
\]

Combining the above two inequalities we can obtain the desired result.
\end{proof}

\begin{lemma}\label{multitau}
 Let $\tau$ be randomly chosen from $\{1,2,\cdots,T\}$ with equal probabilities $p_\tau = \frac{1}{T}$. We have the following estimate:
  \[
  \mathbb{E}[\|\nabla f(x_\tau)\|^2]\leq \frac{\sqrt{G^2+\epsilon d}}{\alpha\sqrt{T}N}\sum_{i=1}^N\mathbb{E}\left[\sum_{t=1}^T\|\nabla f((x_t))\|_{\hat{\eta_t}^{(i)}}^2\right].
  \]
\end{lemma}
\begin{proof}
  By Lemma \ref{ft}, $\mathbb{E}[\|\nabla f(x_\tau)\|^2]\leq \frac{\sqrt{G^2+\epsilon d}}{\alpha\sqrt{T}}\mathbb{E}[\sum_{t=1}^T\|\nabla f(x_t)\|_{\hat{\eta_t}^{(i)}}^2$ holds for any $i$. Hence, the proof is finished.
\end{proof}

\begin{proof}[Proof of Theorem \ref{T2}]
By using the gradient Lipschitz continuity of $f$, it holds that
\[
\begin{split}
\mathbb{E} f(\hat{x}_{t+1}) &\leq \mathbb{E}\left[f(\hat{x}_t) +\langle \nabla f(\hat{x}_t), \Delta_t\rangle + \frac{L}{2}\|\Delta_t\|^2 \right] \\
& = \mathbb{E}\left[f(\hat{x}_t) +\langle \nabla f(x_t), \Delta_t\rangle +\langle \nabla f(\hat{x}_t) - \nabla f(\tilde{x}_t), \Delta_t\rangle +\langle \nabla f(\tilde{x}_t) - \nabla f(x_t), \Delta_t\rangle + \frac{L}{2}\|\Delta_t\|^2 \right]\\
&\leq \mathbb{E}\left[f(\hat{x}_t) +\langle \nabla f(x_t), \Delta_t\rangle +L\|E_t\|\|\Delta_t\| +L\|e_t\|\|\Delta_t\| + \frac{L}{2}\|\Delta_t\|^2 \right]\\
&\leq \mathbb{E}\left[f(\hat{x}_t) +\langle \nabla f(x_t), \Delta_t\rangle +\frac{L(2-\delta_x)}{N}\sum_{i=1}^N \|e_{t}\|\|\Delta_{t}^{(i)}\| + \frac{L(2-\delta_x)(2-\delta_g)}{N}\sum_{i=1}^N \|\Delta_{t}^{(i)}\|^2 \right. \\  &\left.\qquad + \frac{L(2-\delta_x)(2-\delta_g)}{N^2}\sum_{i=1}^N\sum_{j=1}^N\|e_{t}^{(i)}\|\|\Delta_{t}^{(j)}\|\right]\\
&=\mathbb{E}f(\hat{x}_t) +M_t.
\end{split}
\]

Then by summing $t$ from $1$ to $T$, we obtain
\[
\begin{split}
f^*&\leq \mathbb{E}f(x_{T+1}) \leq f(x_1) + \sum_{t=1}^T M_t\\
&\leq f(x_1) +C_4d\alpha\left(\log\left(1+\frac{G^2}{\epsilon d}\right)+\frac{1}{1-\theta}\sum_{t=1}^T (1-\theta_t)\right)- \frac{1-\beta}{2N}\sum_{i=1}^N\sum_{t=1}^T\mathbb{E}\|\nabla f(x_t)\|_{\hat{\eta}_t^{(i)}}^2,
\end{split}
\]

Using Lemma \ref{multitau} and arranging some terms, we have
\[
\begin{split}
\mathbb{E}[\|\nabla f(x_\tau)\|^2]&\leq \frac{\sqrt{G^2+\epsilon d}}{\alpha\sqrt{T}N}\sum_{i=1}^N\mathbb{E}\left[\sum_{t=1}^T\|\nabla f((x_t))\|_{\hat{\eta_t}^{(i)}}^2\right]\\
&\leq \frac{2\sqrt{G^2+\epsilon d}}{\alpha(1-\beta)\sqrt{T}} \left( f(x_1) - f^* +C_4d\alpha\left(\log\left(1+\frac{G^2}{\epsilon d}\right)+\frac{1}{1-\theta}\sum_{t=1}^T (1-\theta_t)\right)\right)\\
&\leq \frac{C_5+C_6\sum_{t=1}^T \frac{1}{t}}{\sqrt{T}},
\end{split}
\]

where 
\[
\begin{split}
C_2 &= \left(\frac{\beta/(1-\beta)}{\sqrt{C_1(1-\gamma)\theta_1}}+1\right)^2,\\
C_4 &= \frac{1}{\sqrt{C_1}(1-\sqrt{\gamma})} \left(\frac{\alpha L(2-\delta_x)(2-\delta_g)}{C_1\theta(1-\sqrt{\gamma})^2\delta_x\delta_g} + \frac{2C_2G}{\sqrt{\theta}}\right),\\
C_5 &= \frac{2\sqrt{G^2+\epsilon d}}{\alpha(1-\beta)}\left(f(x_1) - f^* + C_4d\alpha\log\left(1+\frac{G}{\epsilon d}\right)\right),\\
C_6 &= \frac{2\sqrt{G^2+\epsilon d}C_4 d}{(1-\beta)(1-\theta)}.\\
\end{split}
\]
\end{proof}
